# Supplementary material for: Uncovering Logit Suppression Vulnerabilities in LLM Safety Alignment
Source: arXiv:2405.13068 source file (2026-04-18)
Supplement: Supplementary file 1 [file categories.tex]

%\vspace{3em}
\section{Detailed Explanation of Denial Pattern Categorization}
\label{app:tax-explain}
